# Supplementary material for: Perceptual Grouping in Contrastive Vision-Language Models
Source: arXiv:2210.09996 source file (2023-08-22)
Supplement: Supplementary file 1 [file jaccard-cityscapes.tex]

\begin{table}[ht]
\begin{minipage}{0.38\linewidth}
\scalebox{0.90}{
\centering

\begin{tabular}{l|c}
\toprule
Method                           & JS   \\ \midrule
IIC \cite{Ji2019InvariantIC}     & 6.4  \\
MDC \cite{cho2021picie}        & 7.1  \\
PiCIE \cite{cho2021picie}      & 12.3 \\
STEGO \cite{hamilton2022unsupervised} & 21.0 \\ \midrule
\modelname (ours)                & 22.3 \\ \bottomrule
\end{tabular}}
\end{minipage}
\hspace{0.5em}
\begin{minipage}{0.60\linewidth}
% \vspace{1.2em}
\caption{{\bf Performance of prior unsupervised segmentation models.} The Jaccard Similarity (JS) on the Cityscapes Dataset 27 class segmentation setup followed in \cite{hamilton2022unsupervised} is reported. We note how \modelname exhibits competitive performance even against models containing architectural components specialized for segmentation such as CRFs.}
\label{table:app-unsupervised-segmentation}
\end{minipage}
\end{table}
