# Supplementary material for: Perceptual Grouping in Contrastive Vision-Language Models
Source: arXiv:2210.09996 source file (2023-08-22)
Supplement: Supplementary file 2 [file table-more-results.tex]

% \vspace{-0.3cm}
\begin{table*}[t]
\begin{minipage}{0.65\textwidth}
\small
\centering
\scalebox{1.0}{
%  1 is the default, change whatever you need
\begin{tabular}{l|c|c}
    \toprule
   & dataset & \small{COCO (80 objects)}\\
   \shline
    GroupViT \citet{Xu2023LearningOS} &\multirow{3}{*}{\small{CC-12M}} & 17.7 \\
    OVS \citet{Xu2023LearningOS} $^\dagger$& & 25.1 \\
    \modelname & & \textbf{28.5} \\ 
    \hline
    GroupViT \citet{xu2022groupvit} & \small{CC-12M, YFCC-100M} & 24.3 \\
    \modelname & \datasetname-134M & 32.0 \\ 
   \bottomrule
\end{tabular}}
\end{minipage}
\begin{minipage}{0.30\textwidth}
% \vspace{-0.5em}
\caption{ \textbf{Segmentation of foreground objects.} Numbers are mean IoU across 80 foreground classes in COCO. $^\dagger$ OVS is trained on filtered subset of CC-12M.}
\label{table:more-segmentation}
\end{minipage}

\vspace{-0.1em}
\end{table*}

% ALIGN Results 8/30/2022
% Pool     IN1K ZS	VOC	COCO	ADE-20K
% Avg (baseline)    49.74	29.68	14.36	7.52
% Max   45.87	33.54	15.68	7.23
