# Supplementary material for: Perceptual Grouping in Contrastive Vision-Language Models
Source: arXiv:2210.09996 source file (2023-08-22)
Supplement: Supplementary file 3 [file table-more-results-old.tex]

% \vspace{-0.3cm}
\begin{table*}[t]
\begin{minipage}{0.75\textwidth}
\small
\centering
\scalebox{0.9}{
\def\arraystretch{1.2}%  1 is the default, change whatever you need
\begin{tabular}{l|cc|cc|cc}
    \toprule
   & arch & dataset & \small{ADE20K} & \small{COCO} & \small{PASCAL VOC} & \small{COCO $^\ddagger$}\\
   \shline
    GroupViT \citet{xu2022groupvit}  & ViT & \multirow{4}{*}{\small{CC-12M}} & & & 41.1 & \\
    GroupViT \citet{Xu2023LearningOS}& ViT & & & & 40.2 & 17.7 \\
    OVS \citet{Xu2023LearningOS} $^*$& ViT & & & & 53.8 & 25.1 \\
    \modelname                       & ViT & & 13.1 & 23.8 & \textbf{50.8} & \textbf{27.7} \\ 
   \hline
    ALIGN $^\dagger$ & CNN & \multirow{3}{*}{\small{\datasetname-134M}} & 7.5 & 14.4 & 29.7 & \\
    CLIP $^\dagger$ & ViT &  & 5.1 & 8.0 & 18.1 & \\
    \modelname & ViT &  & \textbf{13.5} & \textbf{25.5} & \textbf{52.2} \\
   \hline  % 13.54 / 25.52 / (average across 3 runs)
    ALIGN \citet{ghiasi2021simple} & CNN & \small{ALIGN-1800M} & 9.7 & 15.6 & & \\
    CLIP \citet{radford2021clip} & ViT & \small{CLIP-400M} & 5.8 & 8.7 & 16.4  & \\
    GroupViT \citet{xu2022groupvit} & ViT & \small{CC-12M, YFCC-100M} & & & 52.3 & 24.3 \\
    %GroupViT \citet{xu2022groupvit} & ViT & \small{CC-12M, YFCC-100M} & &  24.3 & 52.3  \\
   \bottomrule
\end{tabular}}
\end{minipage}
%
\begin{minipage}{0.24\textwidth}
% \vspace{-0.5em}
\caption{ \textbf{More results comparisons.} Numbers are mean IoU. $^\dagger$ indicates our implementation. COCO $^\dagger$ use only 80 object classes. $^*$ OVS is trained on filtered subset of CC12M.}
\label{table:more-segmentation}
\end{minipage}

\vspace{-0.1em}
\end{table*}

% ALIGN Results 8/30/2022
% Pool     IN1K ZS	VOC	COCO	ADE-20K
% Avg (baseline)    49.74	29.68	14.36	7.52
% Max   45.87	33.54	15.68	7.23
